# Supplementary material for: Superior Frequency Stability and Long-Lived State-Swapping in Cubic-SiC Mechanical Mode Pairs
Source: arXiv:2507.05646 ancillary file (2025-07-08)
Supplement: Supplementary file 1 [file Supplemental_Information.pdf]

# Superior Frequency Stability and Long-Lived State-Swapping in Cubic-SiC Mechanical Mode Pairs

Huanying Sun<sup>1,\*</sup>, Yanlin Chen<sup>1,2,3,\*</sup>, Qichun Liu<sup>1,\*</sup>, Haihua Wu,<sup>1</sup> Yuqing Wang,<sup>1</sup> Tiefu Li,<sup>4,1,†</sup> and Yulong Liu<sup>1,2,3,‡</sup>

<sup>1</sup>Beijing Key Laboratory of Fault-Tolerant Quantum Computing,  
Beijing Academy of Quantum Information Sciences, Beijing 100193, China

<sup>2</sup>Beijing National Laboratory for Condensed Matter Physics,  
Institute of Physics, Chinese Academy of Sciences, Beijing 100190, China

<sup>3</sup>University of Chinese Academy of Sciences, Beijing 100049, China

<sup>4</sup>School of Integrated Circuits and Frontier Science Center for  
Quantum Information, Tsinghua University, Beijing 100084, China

(Dated: July 7, 2025)

## SUPPLEMENTAL NOTE 1 - VIBRATION EQUATION OF MEMBRANE RESONATOR

### A. Free bending vibration of plates under tensile: the equation of motion under nonuniform stress

Understanding the underlying mechanisms of mode breaking in the square membrane is essential for realizing its potential applications. In this section, we derive the vibration equation governing the square membrane and provide the analytical expressions for its eigen frequencies. In our analysis, we adopt the following assumptions about the membranes: (1) The membrane is flexible, linearly elastic, and subject to tension that remains within the tangent plane of its surface. In addition, the membrane undergoes relatively small deformations. (2) Due to their thin structure and significant internal stresses, the bending effects in membranes are negligible. A membrane under tensile stresses is illustrated in Supplemental Fig. 1.

In the plane of the membrane, the stress matrix can be expressed as:  $\begin{pmatrix} \sigma_x & 0 \\ 0 & \sigma_y \end{pmatrix}$ . The equilibrium equations for the membrane can be readily derived as follows:

$$\begin{aligned} & \Delta y [\sigma_x(x + \Delta x, y) \sin(\alpha) - \sigma_x(x, y) \sin(\beta)] \\ & + \Delta x [\sigma_y(x, y + \Delta y) \sin(\delta) - \sigma_y(x, y) \sin(\gamma)] \\ & = \rho(\Delta x \Delta y) \cdot u_{tt} \end{aligned} \quad (\text{S.1})$$

Based on the geometric relationships between the dis-

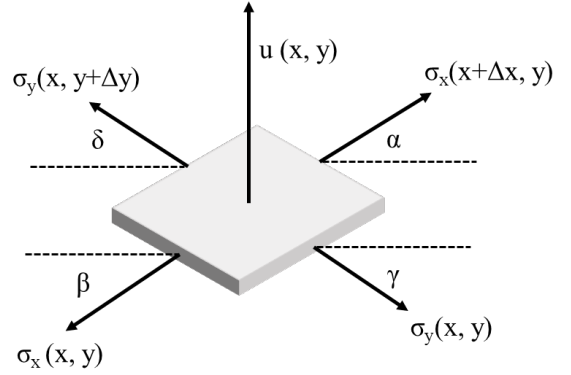

Supplemental Fig. 1. The diagram of a membrane subjected to tensile stresses.  $\sigma_x(x, y)$  and  $\sigma_x(x + \Delta x, y)$  represent the tensile stresses acting along the x-direction, while  $\sigma_y(x, y)$  and  $\sigma_y(x, y + \Delta y)$  depict the tensile action in the y-direction.  $\alpha, \beta, \delta$  and  $\gamma$  indicate the angles between the stresses and the horizontal plane, respectively.

placement and the angles, we obtain the following:

$$\begin{aligned} \sin(\alpha) &= \alpha = \tan(\alpha) = u_x(x + \Delta x, y) \\ \sin(\beta) &= \beta = \tan(\beta) = u_x(x, y) \\ \sin(\delta) &= \delta = \tan(\delta) = u_y(x, y + \Delta y) \\ \sin(\gamma) &= \gamma = \tan(\gamma) = u_y(x, y) \end{aligned} \quad (\text{S.2})$$

By substituting Eq. (S.2) into Eq. (S.1), Eq. (S.1) is transformed into the following form:

$$[\sigma_x(x + \Delta x, y)u_x(x + \Delta x, y) - \sigma_x(x, y)u_x(x, y)]\Delta y \quad (\text{S.3})$$

$$+ [\sigma_y(x, y)u_y(x + \Delta x, y) - \sigma_y(x, y)u_y(x, y)]\Delta x \quad (\text{S.4})$$

$$= \rho \cdot (\Delta x \Delta y) u_{tt} \quad (\text{S.5})$$

Next, we divide both sides of the equation by  $\rho \Delta x \Delta y$

\* These authors contributed equally to this work.

† litf@tsinghua.edu.cn

‡ liuyul@baqis.ac.cn

simultaneously, we get:

$$u_{tt} = \frac{1}{\rho} \left[ \frac{\sigma_x(x + \Delta x, y)u_x(x + \Delta x, y) - \sigma_x(x, y)u_x(x, y)}{\Delta x} + \frac{\sigma_y(x, y)u_y(x + \Delta x, y) - \sigma_y(x, y)u_y(x, y)}{\Delta y} \right] \quad (\text{S.6})$$

As  $\Delta x$  and  $\Delta y$  approach 0, the above equation reduces to the following form:

$$u_{tt} = \frac{1}{\rho} \left[ \frac{(\partial \sigma_x \cdot u_x)}{\partial x} + \frac{(\partial \sigma_y \cdot u_y)}{\partial y} \right] \quad (\text{S.7})$$

$$= \frac{1}{\rho} \left[ \frac{\partial}{\partial x} \left( \sigma_x \frac{\partial u}{\partial x} \right) + \frac{\partial}{\partial y} \left( \sigma_y \frac{\partial u}{\partial y} \right) \right] \quad (\text{S.8})$$

When the stress distribution in the x- and y-directions are being of uniform, the equation simplifies to the following form:

$$\sigma_x \frac{\partial^2 u}{\partial x^2} + \sigma_y \frac{\partial^2 u}{\partial y^2} - \rho \frac{\partial^2 u}{\partial t^2} = 0 \quad (\text{S.9})$$

The  $u(x, y, t)$  can be written as  $u(x, y, t) = X(x) \cdot Y(y) \cdot T(t)$ . Putting this expression into the original equation, and let  $c_x = \sqrt{\frac{\sigma_x}{\rho}}$ ,  $c_y = \sqrt{\frac{\sigma_y}{\rho}}$ , then we obtain:

$$\frac{T_{tt}(t)}{T(t)} = c_x^2 \frac{X_{xx}(x)}{X(x)} + c_y^2 \frac{Y_{yy}(y)}{Y(y)} = \text{constant} = -\omega^2 \quad (\text{S.10})$$

Equation (S.10) can be written as three independent ordinary differential equations:

$$\begin{cases} T_{tt}(t) + \omega^2 T(t) = 0 \\ X_{xx}(x) + \left(\frac{\omega}{c_x}\right)^2 X(x) = 0 \\ Y_{yy}(y) + \left(\frac{\omega}{c_y}\right)^2 Y(y) = 0 \end{cases} \quad (\text{S.11})$$

It is easy to get the solution of the time-dependent equation, that is:

$$T(t) = A \sin(\omega t) + B \cos(\omega t) \quad (\text{S.12})$$

where  $A, B$  are coefficients to be determined by the initial conditions. Usually, we are more concerned with the displacement distribution of the membrane in the x, y directions, while the time-dependent term does not affect the spatial distribution. Similarly, the solution along the x-direction could be expressed as:

$$X(x) = C \sin\left(\frac{\omega_x}{c_x} x\right) + D \cos\left(\frac{\omega_x}{c_x} x\right) \quad (\text{S.13})$$

Here, the coefficients  $C$  and  $D$  are determined by the boundary conditions. For a membrane, the general boundary conditions are fixed at both ends, i.e.,  $u = 0$  at

$x = 0, L$ . Applying these conditions yields the following result:

$$\frac{\omega_x}{c_x} \cdot L = m\pi, \quad m = 1, 2, 3, \dots \quad (\text{S.14})$$

Similar result can be obtained for the case of the y-direction:

$$\frac{\omega_y}{c_y} \cdot L = n\pi \quad n = 1, 2, 3, \dots \quad (\text{S.15})$$

Due to  $\omega_x^2 + \omega_y^2 = \omega^2$ , the resonance frequency can be obtained:

$$\omega^2 = \left(\frac{\pi}{L}\right)^2 \left[ \frac{\sigma_x}{\rho} m^2 + \frac{\sigma_y}{\rho} n^2 \right] \quad (\text{S.16})$$

By simplifying this equation, the eigenfrequency can be expressed as:

$$\frac{\omega_{mn}}{2\pi} = \frac{1}{2L} \sqrt{\frac{\sigma_x m^2 + \sigma_y n^2}{\rho}} \quad (\text{S.17})$$

## B. Free bending vibration of plates under tensile: the equation of motion under uniform stress

Consider the equation of the vibration of a membrane under stress:

$$\sigma \nabla^2 u = \rho \frac{\partial^2 u}{\partial t^2} \quad (\text{S.18})$$

From the equation, through the split-variable method, the form of the solution can be written as:

$$u(x, y, t) = u(x, y) \cos(\omega t) \quad (\text{S.19})$$

As the vibrations in the x, y directions are uncoupled, vibrational morphology can be written:

$$u(x, y) = \sum_{m=0}^{\infty} \sum_{n=0}^{\infty} \sin\left(\frac{m\pi x}{L}\right) \sin\left(\frac{n\pi y}{L}\right) \quad (\text{S.20})$$

Then we have:

$$\frac{\partial^2 u}{\partial x^2} = -\left(\frac{m\pi}{L}\right)^2 u(x, y) \cos(\omega t) = -\left(\frac{m\pi}{L}\right)^2 u(x, y, t) \quad (\text{S.21})$$

$$\frac{\partial^2 u}{\partial y^2} = -\left(\frac{n\pi}{L}\right)^2 u(x, y) \cos(\omega t) = -\left(\frac{n\pi}{L}\right)^2 u(x, y, t) \quad (\text{S.22})$$

And

$$\frac{\partial^2 u}{\partial t^2} = -\omega^2 u(x, y) = -\omega^2 u(x, y, t) \quad (\text{S.23})$$

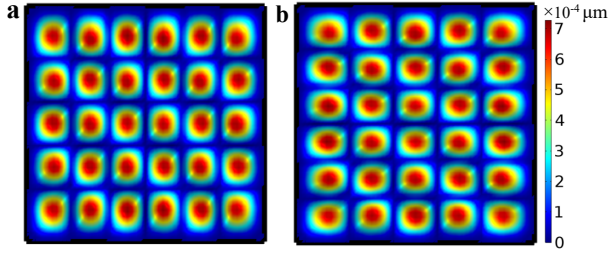

Supplemental Fig. 2. Surface displacement patterns for **a** mode(6,5) and **b** mode(5,6).

Put Eq. (S.21), Eq. (S.22) and Eq. (S.23) into Eq. (S.18), we get:

$$\sigma[-(\frac{m\pi}{L})^2 - (\frac{n\pi}{L})^2]u(x, y, t) + \rho\omega^2 u(x, y, t) = 0 \quad (\text{S.24})$$

We get:

$$\rho\omega^2 = \sigma[(\frac{m\pi}{L})^2 + (\frac{n\pi}{L})^2] \quad (\text{S.25})$$

Finally, we get:

$$\frac{\omega_{mn}}{2\pi} = \frac{1}{2L} \sqrt{\frac{\sigma}{\rho}} \sqrt{m^2 + n^2} \quad (\text{S.26})$$

## SUPPLEMENTAL NOTE 2 - EXPERIMENTAL AND FES RESULTS OF SiC MEMBRANE RESONATOR

The experimental and Finite Element Simulation (FES) results for 57 mechanical modes at room temperature are shown in Supplemental Table 1, with mode indices determined by FES. The data show great agreement between experimental and simulated results. Surface displacement patterns exhibit multiple maxima along the x- and y-axes, governed by their mode indices. The characteristic mode shapes of mode(6,5) and mode(5,6), discussed in Fig. 2b of the main text, are presented in Supplemental Fig. 2.

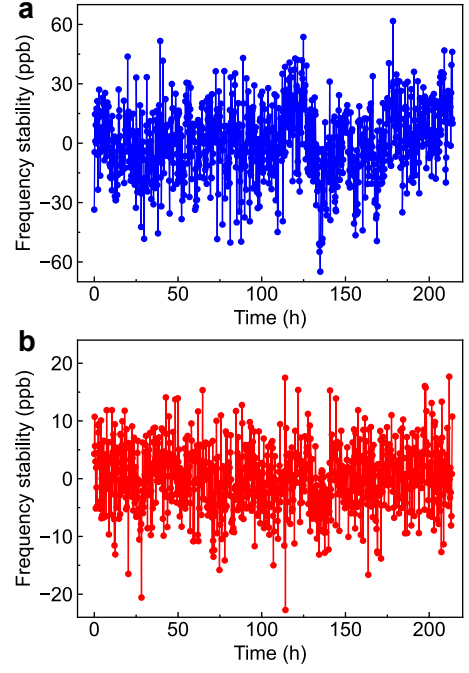

Supplemental Fig. 3. Frequency stability versus time for **a** mode(3,1) and **b** mode(1,3).

The SiC membrane exhibits superior frequency stability, quantified by the relative frequency deviation  $(f - f_0)/f_0$ , where  $f$  is the measured frequency and  $f_0$  is the nominal resonance frequency under reference conditions. As shown in Supplemental Fig. 3, the frequency stability was monitored over a 214-hour period at 10 mK, revealing deviations as low as tens of parts per billion (ppb) for the degeneracy-broken pairs. This remarkable stability at cryogenic temperatures is attributed to the superior thermal conductivity and ultralow mechanical dissipation of SiC, underscoring its potential applications in quantum storage and quantum state manipulation.

Supplemental table 1. Experimental and Finite Element Simulation (FES) results of the SiC membrane resonator at room temperature.

| Number | $f_{\text{Exp.}}$ (kHz) | Quality factor<br>( $\times 10^4$ ) | $f_{\text{FEM}}$ (kHz) | m | n | $m^2 + n^2$ |
|--------|-------------------------|-------------------------------------|------------------------|---|---|-------------|
| 1      | 390.03                  | 2.58                                | 390.02                 | 1 | 1 | 2           |
| 2      | 614.84                  | 23.00                               | 616.67                 | 2 | 1 | 5           |
| 3      | 618.55                  | 18.70                               | 616.67                 | 1 | 2 | 5           |
| 4      | 780.01                  | 50.39                               | 780.03                 | 2 | 2 | 8           |
| 5      | 868.70                  | 4.13                                | 872.1                  | 3 | 1 | 10          |
| 6      | 875.54                  | 2.26                                | 872.1                  | 1 | 3 | 10          |
| 7      | 992.16                  | 28.60                               | 994.35                 | 3 | 2 | 13          |
| 8      | 996.86                  | 12.60                               | 994.35                 | 2 | 3 | 13          |
| 9      | 1132.24                 | 6.56                                | 1137.1                 | 4 | 1 | 17          |
| 10     | 1141.79                 | 11.16                               | 1137.1                 | 1 | 4 | 17          |
| 11     | 1170.43                 | 34.85                               | 1170.0                 | 3 | 3 | 18          |
| 12     | 1229.68                 | 65.40                               | 1233.3                 | 4 | 2 | 20          |
| 13     | 1237.29                 | 79.30                               | 1233.3                 | 2 | 4 | 20          |
| 14     | 1376.74                 | 54.35                               | 1378.9                 | 4 | 3 | 25          |
| 15     | 1381.68                 | 56.10                               | 1378.9                 | 3 | 4 | 25          |
| 16     | 1412.77                 | 39.60                               | 1406.2                 | 5 | 1 | 26          |
| 17     | 1400.03                 | 33.36                               | 1406.2                 | 1 | 5 | 26          |
| 18     | 1480.04                 | 49.30                               | 1485.1                 | 5 | 2 | 29          |
| 19     | 1490.92                 | 56.90                               | 1485.1                 | 2 | 5 | 29          |
| 20     | 1560.42                 | 105.93                              | 1560.1                 | 4 | 4 | 32          |
| 21     | 1604.80                 | 57.80                               | 1608.1                 | 5 | 3 | 34          |
| 22     | 1612.59                 | 45.10                               | 1608.1                 | 5 | 3 | 34          |
| 23     | 1669.93                 | 41.80                               | 1677.5                 | 6 | 1 | 37          |
| 24     | 1685.52                 | 39.40                               | 1677.5                 | 1 | 6 | 37          |
| 25     | 1737.70                 | 60.20                               | 1744.2                 | 6 | 2 | 40          |
| 26     | 1752.01                 | 74.81                               | 1744.2                 | 2 | 6 | 40          |
| 27     | 1763.72                 | 48.50                               | 1765.9                 | 5 | 4 | 41          |
| 28     | 1769.23                 | 47.20                               | 1765.9                 | 4 | 5 | 41          |
| 29     | 1845.05                 | 60.40                               | 1850.0                 | 6 | 3 | 45          |
| 30     | 1856.27                 | 61.20                               | 1850.0                 | 3 | 6 | 45          |
| 31     | 1950.83                 | 176.00                              | 1950.1                 | 5 | 5 | 50          |
| 32     | 1959.43                 | 21.20                               | 1950.1                 | 7 | 1 | 50          |
| 33     | 1941.17                 | 43.68                               | 1950.1                 | 1 | 7 | 50          |
| 34     | 1985.82                 | 52.94                               | 1988.7                 | 6 | 4 | 52          |
| 35     | 1993.53                 | 79.80                               | 1988.7                 | 4 | 6 | 52          |
| 36     | 1999.69                 | 59.10                               | 2007.7                 | 7 | 2 | 53          |
| 37     | 2017.19                 | 33.66                               | 2007.7                 | 2 | 7 | 53          |
| 38     | 2093.94                 | 29.00                               | 2100.3                 | 3 | 7 | 58          |
| 39     | 2108.62                 | 50.80                               | 2100.3                 | 7 | 3 | 58          |
| 40     | 2151.71                 | 66.40                               | 2153.9                 | 6 | 5 | 61          |
| 41     | 2158.30                 | 53.34                               | 2153.9                 | 5 | 6 | 61          |
| 42     | 2213.14                 | 8.72                                | 2223.5                 | 7 | 4 | 65          |
| 43     | 2234.39                 | 23.10                               | 2223.5                 | 4 | 7 | 65          |
| 44     | 2264.86                 | 71.10                               | 2274.2                 | 8 | 2 | 68          |
| 45     | 2285.43                 | 71.10                               | 2274.2                 | 2 | 8 | 68          |
| 46     | 2341.01                 | 57.80                               | 2340.2                 | 6 | 6 | 72          |
| 47     | 2366.62                 | 95.52                               | 2356.4                 | 3 | 8 | 73          |
| 48     | 2370.18                 | 53.80                               | 2372.4                 | 7 | 5 | 74          |
| 49     | 2378.05                 | 59.85                               | 2372.4                 | 5 | 7 | 74          |
| 50     | 2460.91                 | 73.89                               | 2466.8                 | 8 | 4 | 80          |
| 51     | 2475.89                 | 46.35                               | 2466.8                 | 4 | 8 | 80          |
| 52     | 2486.13                 | 13.90                               | 2497.4                 | 9 | 1 | 82          |
| 53     | 2510.02                 | 27.30                               | 2497.4                 | 1 | 9 | 82          |
| 54     | 2532.32                 | 29.22                               | 2542.7                 | 6 | 7 | 85          |
| 55     | 2540.76                 | 51.80                               | 2542.7                 | 7 | 6 | 85          |
| 56     | 2547.83                 | 36.72                               | 2542.7                 | 9 | 2 | 85          |
| 57     | 2555.88                 | 36.70                               | 2542.7                 | 2 | 9 | 85          |
